# Supplementary material for: Topological Defect Mediated Helical Phase Reorientation by Uniaxial Stress
Source: arXiv:2512.06481 source file (2025-12-06)
Supplement: Supplementary file 1 [file SI_v11-PRL-shortened_arxiv.pdf]

**Topological Defect Mediated Helical Phase Reorientation by Uniaxial Stress**

Tae-Hoon Kim,[1,] * Haijun Zhao,[1, 2,] * Brandt A. Jensen,[1] Liqin Ke,[1,] † Lin Zhou[1,3,] †

[1] Ames National Laboratory, U.S. Department of Energy, Ames, Iowa 50011, USA

[2] School of Physics, Southeast University, Nanjing 211189, China

[3] Department of Materials Science and Engineering, Iowa State University, Ames, Iowa 50011, USA

* T.K. and H.Z. contributed equally to this work.

† Correspondence to: liqinke@ameslab.gov; linzhou@ameslab.gov

**Section I. Materials and Methods**

The bulk $Co_8Zn_{8.5}Mn_{3.5}$ sample was prepared by first sealing individual metals (all > 99.9% metal basis) in a quartz ampoule backfilled with ultra-high purity argon. The ampoule was heated at 1000 ℃ for 12 hours, then cooled to 925 ℃ by 1 ℃/hr and held for 96 hours followed by water quenching. Magnetic properties were measured using a Quantum Design VersaLab$^{TM}$ vibrating sample magnetometer. A thin polycrystalline piece was polished and the sample dimensions were greater than 5:1 aspect ratio. The sample was cooled under an applied field of H = 20 Oe with a rate of 2 K/min. The $Co_8Zn_{8.5}Mn_{3.5}$ sample show a Curie temperature of 335 K, and magnetization of 0.20 μB/f.u. under an applied field of H = 20 Oe.

A (001) thin plate with [110] lateral orientation was lifted out by using a focused ion beam (FIB, FEI Helios NanoLab G3) instrument. The TEM specimen was transferred on a push-to-pull (PTP) device and both ends of the specimen were welded by carbon deposition. Low-kV Ga ion imaging was performed to prevent Ga-ion-induced beam damage during the transfer process. The *in-situ* LTEM tensile testing was performed on an FEI Tecnai F20 TEM using a Hysitron PI 95 TEM PicoIndenter. The LTEM video was recorded at 10 fps. The geometry of the sample and calculation procedure of strain and stress are described in Fig. S2. The strain ($\varepsilon$) was calculated by dividing the measured displacement of the gap between fixed and pulled parts of PTP device by the length ($L_0$) of thinned region at the center. The stress applied to the sample ($\sigma$) was calculated by subtracting the portion of the PTP device ($P_{PTP}$ = 150 N/m, the spring stiffness) from the experimentally measured force. Consequently, the stress-strain curve was obtained (Fig. S1B). The quantitative in-plane magnetizations of LTEM Fresnel images are analyzed by a phase-retrieval QPt software on the basis of the transport of intensity equation [1].

**Figure S1**

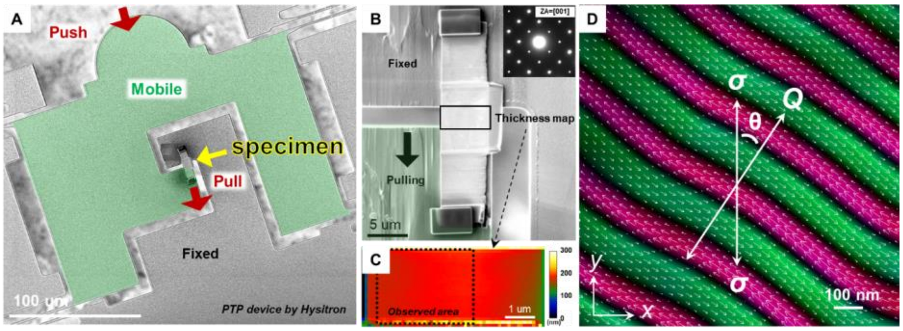


**Fig. S1 The prepared TEM sample on the PTP device for in-situ tensile testing**. (A) Tensile stress is applied to the sample by pushing the semi-circular part of the PTP device. The mobile part is shown in green color. (B) The TEM sample was loaded on PTP device. (C) The thickness map of the sample shows an overall 190 nm thickness. The boxed area was observed for experiments. (D) In-plane magnetization map of helical phase showing the geometric relationship between $Q$, applied stress ($\sigma$), angle between $Q$ and $\sigma$ ($\theta$), and x and y coordinates. Small arrows in helices indicate magnetization direction.

**Figure S2**

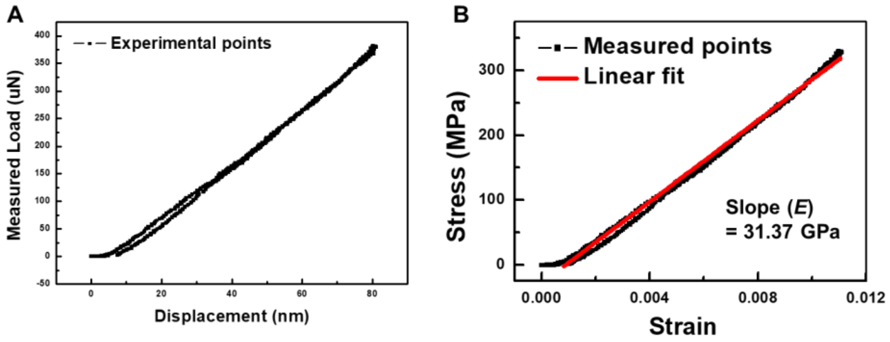


**Fig. S2** (A) Measured displacement of PTP device and force during in-situ tensile testing (B) Calculated stress-strain curve during in-situ tensile testing. The tensile testing wasco nducted under elastic region and Young's modulus is 31.37 GPa.

**Figure S3**

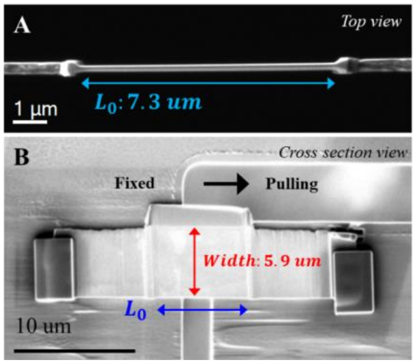


**C**

*Strain*

$$\boldsymbol{\varepsilon} = \frac{\Delta L}{L_0} = \frac{Measured\ displacment}{L_0}$$

*Stress*

$$\boldsymbol{\sigma} = \frac{F}{A_0} = \frac{Measrued\ force\ - \Delta L \times PTP\ Stiffness^{*}}{Width \times thickness^{*}}$$

$^{*}$ $PTP\ stiffness: 150\ N/m$

$^{*}$ $Thickness: 190\ nm$

**Fig. S3 Measured parameters for strain and stress calculation. (A)** Top view of TEM sample before landing on PTP device. The thinned area on center, where strain will be concentrated, has 7.3 um length ($L_0$). **(B)** TEM sample placed on PTP device. Stress area ($A_0$) has 5.9 um width and 190 nm thickness (Fig. 1D). **(C)** Strain and stress calculati on procedures are summarized.

**Section II. Theoretical analysis**

A. **Anisotropic DMI theory**

Phenomenologically, the magnetic system's behavior is captured by the free energy functional, which, to second order in magnetization gradients, in most general form, is expressed as [2] :

$$F = F_{ex} + F_{DMI} + F_h + F_a = \int_V (A_{ij}\partial_i \boldsymbol{m} \cdot \partial_j \boldsymbol{m} + D_{ijk} m_i \partial_j m_k)\ \mathrm{d}\tau + F_h + F_a. \quad \text{(S1)}$$

Here, Einstein's summation convention is applied. $A_{ij}$ and $D_{ijk}$ are exchange stiffness tensor and DMI tensor, respectively. $F_h$ describes contribution of external magnetic field. $F_a$ is anisotropy energy including dipolar interactions.

In cubic noncentrosymmetric chiral magnets like MnSi, FeGe, and $Co_8Zn_xMn_{12\text{-}x}$, the exchange stiffness and DMI become isotropic in the absence of strain, where $A_{ij} = A\delta_{ij}$ and $D_{ijk} = D\epsilon_{ijk}$, with $\epsilon_{ijk}$ being the Levi-Civita symbol. This simplifies the energy functional to:

$$F = \int_V (A\partial_i \boldsymbol{m} \cdot \partial_i \boldsymbol{m} + D\boldsymbol{m} \cdot \boldsymbol{\nabla} \times \boldsymbol{m})\ \mathrm{d}\tau + F_h + F_a, \quad \text{(S2)}$$

This form constitutes the widely adopted standard model [3–6].

For the helical phase, where the external magnetic field is absent ($F_h = 0$) and anisotropy energy $F_a$ is weak enough to be neglected, minimizing the total energy given by Eq. (3) yields an optimal $Q = |\mathrm{D}|/(2A)$ and a minimum helix energy $E_{\mathrm{H}}^0 = -\frac{D^2}{4\mathrm{A}}$ [4,6]. Notably, both Q and $E_{\mathrm{H}}^0$ vanish when $D = 0$, indicating that the ferromagnetic (FM) state prevails in the absence of DMI. Furthermore, due to the isotropic nature of the exchange and DMI terms, the direction of $\boldsymbol{Q} = (Q_x, Q_y, Q_z)$ can be arbitrarily oriented.

When strain is applied, the isotropy of the exchange stiffness and DMI may be disrupted. Following Ref. [7], we assume that the change in exchange stiffness is negligible, while the strain-

induced anisotropic DMI dominates. In this scenario, the DMI tensor remains antisymmetric, i.e., $D_{ijk}$=-$D_{kji} = D_j$. Neglecting $F_h$ and $F_a$, the energy functional simplifies to:

$$F = \int_V \left[A(\nabla \boldsymbol{m})^2 + D_x L_{yz}^{(x)} + D_y L_{zx}^{(y)}\right] \mathrm{d}\tau \qquad \text{(S3)}$$

where, $L_{jk}^{(i)} = m_k \frac{\partial}{\partial \mathrm{i}} m_j - m_j \frac{\partial}{\partial \mathrm{i}} m_k$ represents the Lifshitz invariant. For simplicity, we have confined the problem to a two-dimensional system.

Assuming a tensile strain $\sigma$ applied along the $\hat{y}$ direction, this leads to a reduction in $D_y$, while $D_x$ remains unaffected, i.e., $D_x = D_y(0) = D$ . Consequently, the DMI becomes anisotropic, which can be effectively characterized by the parameter $\eta(\sigma) = 1 - \frac{D_y(\sigma)}{D}$. Here, η acts as an effective strain parameter that increases from 0 to 1 as the strain $\sigma$ increases.

## B. **Analytical calculation of relation ship between the energy of helical phase and reorientation angel**

The anisotropic DMI theory outlined above enables us to analytically derive the relationship between the energy of the helical phase and the reorientation angle. Consider the magnetic configuration of a single helical state given by:

$$\boldsymbol{M}_{helical}(\boldsymbol{r}) = \boldsymbol{M}_0 e^{i\boldsymbol{Q}\cdot\boldsymbol{r}} + \boldsymbol{M}_0^* e^{-i\boldsymbol{Q}\cdot\boldsymbol{r}}, \qquad \text{(S4)}$$

where $\boldsymbol{M}_0 = 1/2[\boldsymbol{M}_{helical}(0) - i\,\boldsymbol{M}_{helical}(2\pi/Q)]$. Substituting this into the energy functional (Eq. (1)), the free energy is:

$$E = \left[2AQ^2 \boldsymbol{M}_0 \cdot \boldsymbol{M}_0^* + 2iD_x Q_x\left(M_y^* M_z - M_z^* M_y\right) + 2iD_y Q_y (M_z^* M_x - M_x^* M_z)\right]/M_S^2$$

This simplifies to:

$$\mathrm{E} = [\boldsymbol{m}_0^*]^T M_E \boldsymbol{m}_0,$$

where $\boldsymbol{m_0} = \boldsymbol{M_0}/M_s$, and $M_E$ is a matrix given by:

$$M_E = \begin{pmatrix} 2A(Q_x^2 + Q_y^2) & 0 & -2iD_yQ_y \\ 0 & 2A(Q_x^2 + Q_y^2) & 2iD_xQ_x \\ 2iD_yQ_y & -2iD_xQ_x & 2A(Q_x^2 + Q_y^2) \end{pmatrix}$$

The smallest eigenvalue of $M_E$ is

$$\lambda = 2AQ^2 - 2Q\sqrt{D_x^2 sin^2\theta + D_y^2 cos^2\theta} = 2AQ^2 - 2QD\sqrt{1 + \eta(\eta - 2)\cos^2\theta}. \qquad \text{(S5)}$$

where we have used $D_x = D$ and $D_\text{y} = D(1 - \eta)$. Minimizing $\lambda$ with respect to $Q$, and noting that $E = \lambda\boldsymbol{m_0}\cdot\boldsymbol{m}_0^* = \frac{1}{2}\lambda$ (since $|\boldsymbol{m_0}| = 1/\sqrt{2}$), one has

批注 [LZ1]: We need to define $\eta$ ?

$$E_{min} = -\frac{D^2}{4A}[1 + \eta(\eta - 2)\cos^2\theta] \qquad \text{(S6)}$$

The corresponding Q is

$$Q = \frac{D}{2A}\sqrt{1 + \eta(\eta - 2)\cos^2\theta} \qquad \text{(S7)}$$

For $\eta = 0$, i.e., zero strain, $E_{min} = -\frac{D^2}{4A}$, and $Q = \frac{D}{2A}$, consistent with the isotropic case.

As $\eta$ increases, the energy rise $\Delta E_\text{H}(\theta, \eta)$ can be calculated in two scenarios:

(i) For fixed $Q = \frac{D}{2A}$:

$$\Delta E_\text{H}(\theta, \eta) = \frac{D^2}{2A}\left[1 - \sqrt{1 + \eta(\eta - 2)\cos^2\theta}\right] \qquad \text{(S8)}$$

(ii) For relaxed Q given by Eq. (S7):

$$\Delta E_\text{H}(\theta, \eta) = -\frac{D^2}{4A}[1 + \eta(\eta - 2)\cos^2\theta] \qquad \text{(S9)}$$

In practical scenarios, Q often exhibits partial relaxation, positioning the actual energy rise somewhere between these two extreme cases. Notably, both scenarios exhibit a minimum energy value when $\theta = \pi/2$, signifying that Q is perpendicular to the applied strain direction. This observation aligns with experimental findings for large strain conditions, where the helical phase undergoes complete reorientation. Figure 3 addresses a scenario where a strain is abruptly applied, precluding immediate adjustment in the magnetic structure. Consequently, the energy of the helix phase, $E_H$, is approximated using Eq. (S8).

**C. Comparing strain induced magnetocrystalline anisotropy and adjusting of DMI**

Assuming the strain is applied in $\hat{x}$ direction, the magnetocrystalline anisotropy $E_A$ can be written as

$$E_A = -L(1+v)\mathrm{e}_{\mathrm{xx}}\mathrm{S}_{\mathrm{x}}^2 = Km_x^2 \qquad \text{(S10)}$$

Here, $L$ is a coefficient originating from spin-orbit coupling, while $v$ and $e_{xx}$ are Poisson's ratio and strain, respectively. $S_x$ and $m_x$ denote the $x$-component of spin and magnetization, respectively. The sign of $K$ depends on the combination of $L$, $1+v$, and $e_{xx}$, which can be altered by applying either compressive or tensile stress. As shown in Figure S4(A), for positive $K$, $E_A$ minimizes when $m_x = 0$, implying the helical phase's propagation vector Q aligns parallel to the strain direction ($\hat{x}$-axis). Yet, our experiments contradict this, showing Q rotating perpendicular to the applied stress. In the case of negative $K$, $E_A$ can be re-expressed as

$$E_A = K\left(m_x^2 + m_y^2 + m_z^2\right) - Km_y^2 - Km_z^2 = K|m|^2 - Km_y^2 - Km_z^2 \qquad \text{(S11)}$$

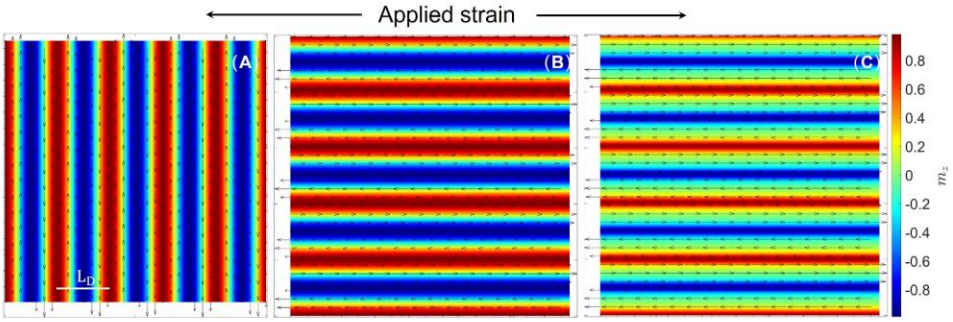


**Fig. S4 Contour plots of ground state magnetic configurations in helical structures after minimizing the strain-induced magnetocrystalline anisotropy energy $\boldsymbol{E_A = Km_x^2}$.** The color scale represents the $z$ component of the magnetization $m_z$, while arrows indicate spin orientations. (**A**) For positive anisotropy constant $K$, $E_A$ minimization requires $m_x = 0$, resulting in the helical phase's propagation vector Q aligning parallel to the strain direction ($x$-axis) - a configuration inconsistent with our experimental observations where Q rotates perpendicular to the applied stress. **(B-C)** For negative $K$ values, $E_A$ minimization can be achieved through two distinct mechanisms: (**B**) When $m_y = 0$ , Q rotates perpendicular to the strain direction, consistent with our experimental findings; (**C**) Minimization of $|m_z|$ leads to peak narrowing ($m_z \approx 1$, red regions) and trough narrowing ($m_z \approx -1$, blue regions), while broadening the intermediate transition regions ($|m_z| \approx 0$) - a feature that contradicts our experimental results.

The first term, $K|m|^2$, represents a constant energy contribution and remains invariant. In two-dimensional systems, the second term ($-Km_y^2$) drives the Q-vector orientation perpendicular to the applied strain through energy minimization when $m_y = 0$, which aligns with our experimental observations (see Fig. S4(B)). However, the third anisotropy term ($-Km_z^2$) creates a theoretical inconsistency by attempting to modify the sinusoidal $m_z$ distribution through preferential energy minimization. This term would induce profile distortion by narrowing both peaks ($m_z \approx 1$) and troughs($m_z \approx -1$) while broadening the intermediate transition regions ($|m_z| \approx 0$) (see Fig. S4(C)), theoretically leading to progressive thinning of helical stripe structures under increased stress conditions—a phenomenon conspicuously absent in our

experimental measurements. This fundamental discrepancy between the model's predictions and empirical data strongly suggests that strain-induced magnetocrystalline anisotropy effects plays an insignificant role in our experiment.

### D. Micromagnetic simulation

The micromagnetic simulation is carried out by numerically integrating the Landau-Lifshitz-Gilbert (LLG) equation:

$$\frac{1+\alpha^2}{\gamma}\frac{\mathrm{d}\mathbf{m}}{\mathrm{d}\tau} = -\mathbf{m} \times \boldsymbol{B}_{\text{eff}} - \alpha\mathbf{m} \times \mathbf{m} \times \boldsymbol{B}_{\text{eff}} \qquad \text{(S12)}$$

Here, $\alpha$ represents the dimensionless damping parameter, $\gamma$ is the gyromagnetic ratio, and $\mathbf{m}$ the unit vector denoting the magnetization direction. The effective magnetic field $\boldsymbol{B}_{\text{eff}}$ is given by:

$$\boldsymbol{B}_{\text{eff}} = -\frac{\partial w}{\mathrm{M_s}\partial\mathbf{m}} + \boldsymbol{B}_{\text{thermal}},$$

where *w* is the energy density given by the integrand of Eq. (S3):

$$w = A(\nabla\boldsymbol{m})^2 + D_x L_{yz}^{(x)} + D_y L_{zx}^{(y)} = A(\nabla\boldsymbol{m})^2 + D[L_{yz}^{(x)} + (1-\eta)L_{zx}^{(y)}] \qquad (S13)$$

The thermal field $\boldsymbol{B}_{\text{thermal}}$ satisfies the condition [7,8]

$$<\boldsymbol{B}_{\text{thermal}}>= 0,$$

and

$$<\boldsymbol{B}_{\text{thermal,i}}(\tau)\boldsymbol{B}_{\text{thermal,j}}(\tau')>=\frac{2\mathrm{k_B T}\alpha}{\mathrm{M_s}\gamma\mathrm{V}}\delta(\tau-\tau')\delta_{ij},$$

which can be written as:

$$\boldsymbol{B}_{\text{thermal}}(\mathrm{T})=\boldsymbol{\eta}\sqrt{\frac{2\mathrm{k_B}T\alpha}{\mathrm{M_s}\gamma \mathrm{V}\Delta\tau}}=\boldsymbol{\eta}\sqrt{\frac{T/T_c}{\Delta\tau}}\sqrt{\frac{2\mathrm{k_B}T_c\alpha}{\mathrm{M_s}\gamma \mathrm{V}}}=\ \boldsymbol{\eta}\frac{\sqrt{t}}{\sqrt{\Delta\tau}}B_c.$$

Here, $\boldsymbol{\eta}$ represents a random vector that is sampled from a standard normal distribution. $T_c$ is the critical temperature above which the helical phase is destroyed. $\mathrm{V}$ is the volume of the unit cell and $\Delta\tau$ is the time step. To determine $B_c$, we initially set $t=1$, and incrementally increase $B_c$ from zero until the system is disrupted. Subsequently, we maintain $B_c$, and adjust the thermal field by varying the effective temperature $t=T/T_c$ from 0 to 1. As expected, lower $t$ requires a greater strain to break and reconnect helices (as well as glide and climb edge dislocations). In Fig. 4, we set $t=0.4$, which is close to the optimal temperature for skyrmion formation. Integration of the LLG equation is executed using our self-developed GPU-accelerated code, employing the sixth-order Runge-Kutta-Fehlberg method, as implemented in MuMax3 [8]. We utilize dimensionless units, which, in contrast to real units, can represent a range of real materials rather than just a specific one. By dividing $D^2/(4A)$ on both side of Eq. (S13), and noting that $A/D=L_D/4\pi$, the equation becomes dimensionless when energy is measured in units of $D^2/(4A)$ and length in unit of $L_D$. For convenience in the simulation, we take $A=1$ and $D=4\pi$. The mesh size is $dx=dy=L_D/16=1/16$. The size of the simulation cell is $16L_D\times 16L_D$. We have conducted additional verifications using a finer mesh and a larger simulation cell, yielding similar results that indicate that errors due to the finite difference method and finite size effects are sufficiently minimal. Periodic boundary conditions are applied in both directions.

The reorientation angle can be varied by either adjusting the direction of strain or rotating the propagation direction of helices. We adjust the direction of strain for calculating the energy of an edge dislocation or helix (Fig. 3), whereas we initiate helices with different propagation directions for micromagnetic simulations of strain-induced reorientation processes (Fig. 4).

**References**


[1] K. Ishizuka and B. Allman, Phase Measurement in Electron Microscopy Using the Transport of Intensity Equation, Microsc. Today **13**, 22 (2005).
[2] L. D. Landau, L. P. Pitaevskii, and E. M. Lifshitz, *Electrodynamics of Continuous Media, Course of Theoretical Physics (Pergamon, Oxford, 1984)*, Vol. 8 (n.d.).
[3] I. E. Dzyaloshinskii, Theory of Helicoidal Structures in Antiferromagnets, III Sov Phys JETP **20**, 665 (1965).
[4] A. O. Leonov et al., Chiral Surface Twists and Skyrmion Stability in Nanolayers of Cubic Helimagnets, Phys. Rev. Lett. **117**, 087202 (2016).
[5] K. M. D. Hals and K. Everschor-Sitte, New Boundary-Driven Twist States in Systems with Broken Spatial Inversion Symmetry, Phys. Rev. Lett. **119**, 127203 (2017).
[6] F. N. Rybakov, A. B. Borisov, S. Blügel, and N. S. Kiselev, New Spiral State and Skyrmion Lattice in 3D Model of Chiral Magnets, New J. Phys. **18**, 045002 (2016).
[7] W. F. Brown, Thermal Fluctuations of a Single-Domain Particle, Phys. Rev. **130**, 1677 (1963).
[8] J. Leliaert, J. Mulkers, J. De Clercq, A. Coene, M. Dvornik, and B. Van Waeyenberge, Adaptively time stepping the stochastic Landau-Lifshitz-Gilbert equation at nonzero temperature: Implementation and validation in MuMax $^3$, AIP Adv. **7**, 125010 (2017).
